# Supplementary material for: Selective Sampling and Mixture Models in Generative Adversarial Networks
Source: arXiv:1802.01568 source file (2018-02-02)
Supplement: Supplementary file 1 [file supplementary.tex]

\begin{figure}[t]
	\begin{tikzpicture}[every node/.style={inner sep=0,outer sep=0}]
	\node (a)
	{\includegraphics[width=\linewidth, totalheight=0.13\linewidth]{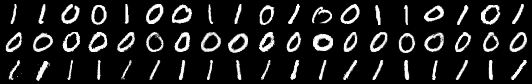}};
	\node (a) [below = 2mm of a.south, anchor=north]
	{\includegraphics[width=\linewidth, totalheight=0.13\linewidth]{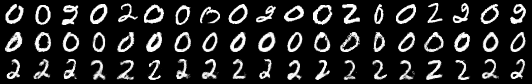}};
	\node (a) [below = 2mm of a.south, anchor=north]
	{\includegraphics[width=\linewidth, totalheight=0.13\linewidth]{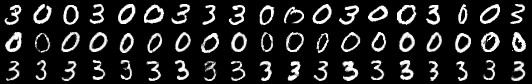}};
	\node (a) [below = 2mm of a.south, anchor=north]
	{\includegraphics[width=\linewidth, totalheight=0.13\linewidth]{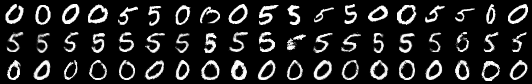}};
	\node (a) [below = 2mm of a.south, anchor=north]
	{\includegraphics[width=\linewidth, totalheight=0.13\linewidth]{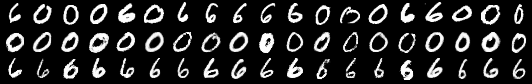}};
	\node (a) [below = 2mm of a.south, anchor=north]
	{\includegraphics[width=\linewidth, totalheight=0.13\linewidth]{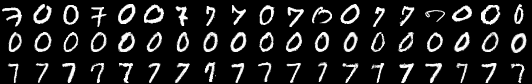}};
	\node (a) [below = 2mm of a.south, anchor=north]
	{\includegraphics[width=\linewidth, totalheight=0.13\linewidth]{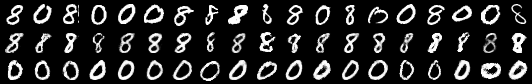}};
	\node (a) [below = 2mm of a.south, anchor=north]
	{\includegraphics[width=\linewidth, totalheight=0.13\linewidth]{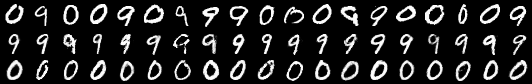}};
	\end{tikzpicture}
	\caption{Successful selective sampling of two digits.}
\end{figure}

\begin{figure}[t]
\begin{tikzpicture}[every node/.style={inner sep=0,outer sep=0}]
	\node (a)
	{\includegraphics[width=\linewidth, totalheight=0.13\linewidth]{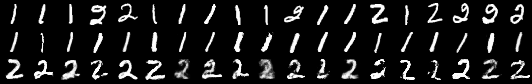}};
	\node (a) [below = 2mm of a.south, anchor=north]
	{\includegraphics[width=\linewidth, totalheight=0.13\linewidth]{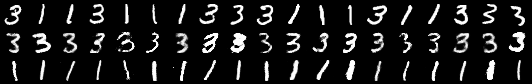}};
	\node (a) [below = 2mm of a.south, anchor=north]
	{\includegraphics[width=\linewidth, totalheight=0.13\linewidth]{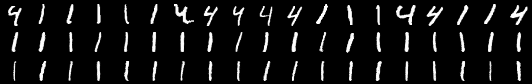}};
	\node (a) [below = 2mm of a.south, anchor=north]
	{\includegraphics[width=\linewidth, totalheight=0.13\linewidth]{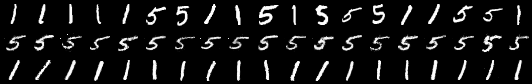}};
	\node (a) [below = 2mm of a.south, anchor=north]
	{\includegraphics[width=\linewidth, totalheight=0.13\linewidth]{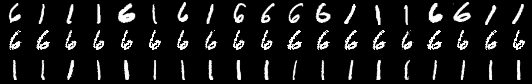}};
	\node (a) [below = 2mm of a.south, anchor=north]
	{\includegraphics[width=\linewidth, totalheight=0.13\linewidth]{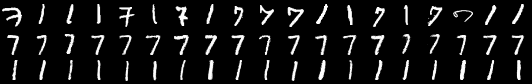}};
	\node (a) [below = 2mm of a.south, anchor=north]
	{\includegraphics[width=\linewidth, totalheight=0.13\linewidth]{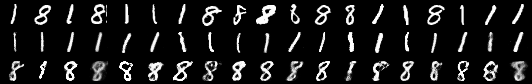}};
	\end{tikzpicture}
	\caption{Successful selective sampling of two digits.}
\end{figure}

\begin{figure}[t]
	\begin{tikzpicture}[every node/.style={inner sep=0,outer sep=0}]
	\node (a)
	{\includegraphics[width=\linewidth, totalheight=0.13\linewidth]{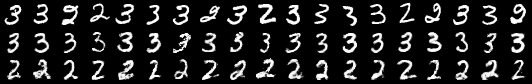}};
	\node (a) [below = 2mm of a.south, anchor=north]
	{\includegraphics[width=\linewidth, totalheight=0.13\linewidth]{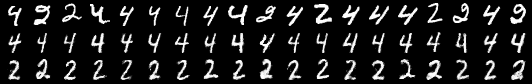}};
	\node (a) [below = 2mm of a.south, anchor=north]
	{\includegraphics[width=\linewidth, totalheight=0.13\linewidth]{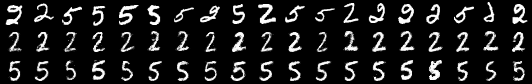}};
	\node (a) [below = 2mm of a.south, anchor=north]
	{\includegraphics[width=\linewidth, totalheight=0.13\linewidth]{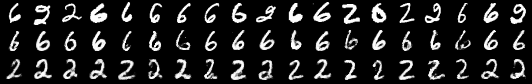}};
	\end{tikzpicture}
	\caption{Successful selective sampling of two digits.}
\end{figure}

\begin{figure}[t]
	\begin{tikzpicture}[every node/.style={inner sep=0,outer sep=0}]
	\node (a)
	{\includegraphics[width=\linewidth, totalheight=0.13\linewidth]{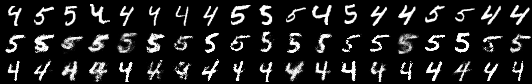}};
	\node (a) [below = 2mm of a.south, anchor=north]
	{\includegraphics[width=\linewidth, totalheight=0.13\linewidth]{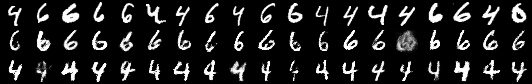}};
	\node (a) [below = 2mm of a.south, anchor=north]
	{\includegraphics[width=\linewidth, totalheight=0.13\linewidth]{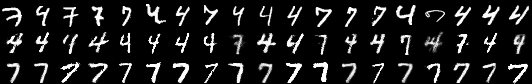}};
	\node (a) [below = 2mm of a.south, anchor=north]
	{\includegraphics[width=\linewidth, totalheight=0.13\linewidth]{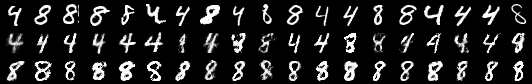}};
	\node (a) [below = 2mm of a.south, anchor=north]
	{\includegraphics[width=\linewidth, totalheight=0.13\linewidth]{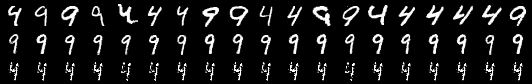}};
	\end{tikzpicture}
	\caption{Successful selective sampling of two digits.}
\end{figure}

\begin{figure}[b]
	\begin{tikzpicture}[every node/.style={inner sep=0,outer sep=0}]
	\node (a)
	{\includegraphics[width=\linewidth, totalheight=0.13\linewidth]{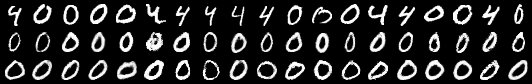}};
	\node (a) [below = 2mm of a.south, anchor=north]
%	{\includegraphics[width=\linewidth, totalheight=0.13\linewidth]{./figures/DIGITS12_DIS1_EPOCH0003399_019.png}};
%	\node (a) [below = 2mm of a.south, anchor=north]
	{\includegraphics[width=\linewidth, totalheight=0.13\linewidth]{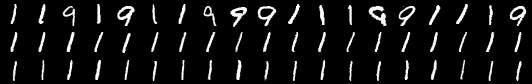}};
	\node (a) [below = 2mm of a.south, anchor=north]
	{\includegraphics[width=\linewidth, totalheight=0.13\linewidth]{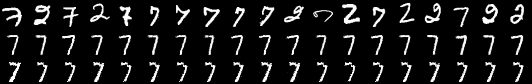}};
	\end{tikzpicture}
	\caption{Examples of failure cases. While the two generators collapse to the same digit, they still maintain different representations to some extent.}
\end{figure}
